# Supplementary material for: Arithmetic Fourier transforms over finite fields: generic vanishing, convolution, and equidistribution
Source: arXiv:2109.11961 source file (2025-09-08)
Supplement: Supplementary file 1 [file appendix-F.tex]

\chapter{Remarks on the early history of Frobenius equidistribution}
\label{ch-history}

\section{Kronecker}

It seems that the story begins with a short paper of
Kronecker~\cite{kronecker} in February 1880, written in honor of
Kummer's 70th birthday. In it, Kronecker states the following theorem
(in translation, but using Kronecker's notation):

\begin{displayquote}
If $F(x)$ is a polynomial function of~$x$, and $\nu_p$ denotes the
number of roots of the congruence $F(x)\equiv 0\bmod{p}$, then the
series
$$
\sum_p\nu_pp^{-1-w},
$$
where~$p$ ranges over all prime numbers, is equivalent as $w\to 0$ to
$\log(1/w)$ multiplied by the number of irreducible factors of~$F(x)$.
\end{displayquote}

It is of some interest (in view of the considerations in
Chapter~\ref{sec-larsen}) that Kronecker's explicit motivation was to
find some criterion for the \emph{irreducibility} of certain
polynomials. He discusses in particular cyclotomic polynomials and the
polynomials whose roots are CM $j$-invariants with given discriminant.

Considering the subsums of his series where $\nu_p$ takes a fixed value,
Kronecker deduces that the densities (``Dichtigkeit''), say $D_k$, of
the sets of primes with this property satisfy the relation
$$
\sum_{k}kD_k=1
$$
if~$F$ is irreducible. For a ``general'' equation of degree~$d$, namely
one with Galois group the full symmetric group~$S_d$, he deduces that
$$
D_k=\frac{1}{k!}\sum_{h=0}^{d-k}\frac{(-1)^h}{h!}.
$$

Interestingly, Kronecker also specifically notes that this density is
almost equal to $e^{-1}/k!$ if $d$ is large and~$k$ relatively
small. This limiting density is none other than the probability that a
Poisson random variable with parameter~$1$ takes the value~$k$
(see~\cite{invariants} for more discussion of this fact and its relation
with random permutations and Deligne--Knop tensor enveloped categories).

Kronecker, as far as we have determined by looking through his works,
did not actually prove the theorem above. 

% From the modern perspective, Kronecker's Theorem is equivalent to the
% following: the limit
% $$
% \lim_{w\to 0}
% $$

\section{Frobenius}

The paper of Kronecker is the explicit starting point of the work of
Frobenius~\cite{frobenius}, which he states was completed already in
November 1880, and communicated to a few people (in particular
Stickelberger and Dedekind) but which did not appear until 1896, shortly
after Hurwitz had communicated to him his own simplifed account in a
letter in January 1896.

Frobenius interprets the number of roots $\nu_p$ as the number of fixed
points of what he calls the associated subtitution of the roots of~$F$,
resulting from the action $x\mapsto x^p$ on these roots. This
substitution is viewed initially only as a conjugacy class in the
symmetric group of~$d=\deg(F)$ letters.

With this interpretation, Kronecker's Theorem is equivalent to
the fact that the limit
$$
\lim_{w\to
  0}\frac{\displaystyle{\sum_p\nu_pp^{-1-w}}}{\displaystyle{\sum_p
    p^{-1-w}}}=
\lim_{w\to
  0}\frac{\displaystyle{\sum_p\nu_pp^{-1-w}}}{\log(1/w)}
$$
(exists and) recovers the multiplicity of the trivial representation in
the linear representation~$\rho$ of the Galois group of~$F$ associated
to the permutation representation of~$S_d$ acting on its roots.  This
can be recognized as a distant ancestor\footnote{\ In the sense of the
  theory of evolution.} of our Proposition~\ref{pr-weyl-sum-bis}.

Using auxiliary polynomials and applying Kronecker's Theorem to them,
Frobenius is able to deduce from these facts the analogue of
Theorem~\ref{th-4}, in the form of the statement that the density of the
set of primes where the associated (Frobenius!) substitution is in a
given conjugacy class of~$S_d$ is equal to the proportion of elements of
the Galois group of~$F$ which are in this conjugacy class, in the
ambient group $S_d$. He further deduces the fact that the $\nu_p$, which
are the values of the character of the representation $\rho$ at
Frobenius classes, ``become equidistributed'' with respect to the
Sato--Tate measure of the Galois group in its representation~$\rho$,
which is parallel to Theorem~\ref{th-3}.

As we have indicated, Frobenius focused in this early part of his paper
on the substitutions given by permutations of the
roots. In~\cite[\S\,3]{frobenius}, Frobenius recounts how he asked
Dedekind about conjecture that any Frobenius substitution must
represented in the Galois group of~$F$ (i.e., the group contains an
element which is conjugate in $S_d$ to the permutation of the
roots). Dedekind established this fact, as explained by Frobenius. But
then Frobenius goes further, by associating the substitution to a prime
ideal above~$p$ by its usual $p$-power action on all integers.

This being established, Frobenius can formulate the conjecture which is
now Chebotarev's Theorem: the equidistribution of Frobenius conjugacy
classes should hold in the Galois group~$G$; this is the counterpart of
the statement which we have only proved partially in Theorem~\ref{th-2}.

\section{Hurwitz, Gassman, Chebotarev and beyond}

Hurwitz did not publish his own account, but his manuscript appeared in
the thesis of F. Gassmann, who further elaborated on parts of it
(see~\cite[p.\,1--5]{gassmann} for the transcription of Hurwitz's
manuscript).

We refer to the excellent survey of Lenstra and
Stevenhagen~\cite{lenstra-stevenhagen} for a detailed look at the
history of the proof of the Chebotarev density theorem, and its impact
on the proof of the reciprocity law of Class Field Theory, There is as
yet no historical presentation of the development of equidistribution
with ``continuous'' groups, but some of the notes and letters between
Serre and Tate~\cite{serre-tate} give an \emph{aperçu} of how some of
these ideas appeared.

%%% Local Variables: 
%%% mode: latex
%%% TeX-master: "convolution-equidistribution"
%%% End: 
